# Supplementary material for: Charge density wave in kagome lattice intermetallic ScV6Sn6
Source: arXiv:2205.04582 ancillary file (2022-06-20)
Supplement: Supplementary file 1 [file ScV6Sn6_CDW_SI_02.pdf]

# Charge density wave in kagome lattice intermetallic $ScV_6Sn_6$

Hasitha W. Suriya Arachchige,[1,*] William R. Meier,[2,†] Madalynn Marshall,[3] Takahiro Matsuoka,[2] Rui Xue,[1] Michael A. McGuire,[4] Raphael P. Hermann,[4] Huibo Cao,[3] and David Mandrus[1,2,4,‡]

[1] *Department of Physics & Astronomy , University of Tennessee Knoxville, Knoxville, Tennessee 37996, USA*
[2] *Materials Science & Engineering Department, University of Tennessee Knoxville, Knoxville, Tennessee 37996, USA*
[3] *Neutron Scattering Division, Oak Ridge National Laboratory, Oak Ridge, Tennessee 37831, USA*
[4] *Materials Science & Technology Division, Oak Ridge National Laboratory, Oak Ridge, Tennessee 37831, USA*

(Dated: June 20, 2022)

## SUPPLEMENTAL MATERIAL

Figure 1 is a optical micrograph of a $ScV_6Sn_6$ crystal. The hexagonal (001) facet faces up with six pyramidal facets around the outside.

### Powder x-ray diffraction

Powder X-Ray Diffraction (PXRD) measurements were performed on ground acid-etched crystals in a Panalytical Empyrean diffractometer with a Cu $K_\alpha$ source. Refinement with JANA2020 [1] (Fig. 2) revealed that $ScV_6Sn_6$ has a $P6/mmm$ $HfFe_6Ge_6$-type structure ($a = 5.47497(8)$ Å, $c = 9.17660(14)$ Å).

### Single crystal x-ray diffraction

Using the ISODISTORT software [3, 4], rhombohedral space groups were selected based on the $\frac{1}{3}\frac{1}{3}\frac{1}{3}$ propagation vector. The space groups $R\bar{3}m$ and $R3m$ resulted in a lower quality refinement and several negative anisotropic displacement parameters. Upon decreasing further in symmetry, a higher quality refinement was achieved with the subsequent space group $R32$, without negative anisotropic displacement parameters. In all these cases the largest displacement mode belongs to the $\frac{1}{3}\frac{1}{3}\frac{1}{3}$ $P_1$ irreducible representation of $P6/mmm$ [3, 4].

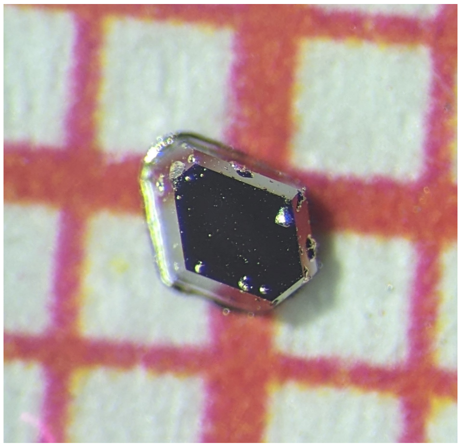

FIG. 1. An optical micrograph of $ScV_6Sn_6$ crystal on a 1 mm grid.

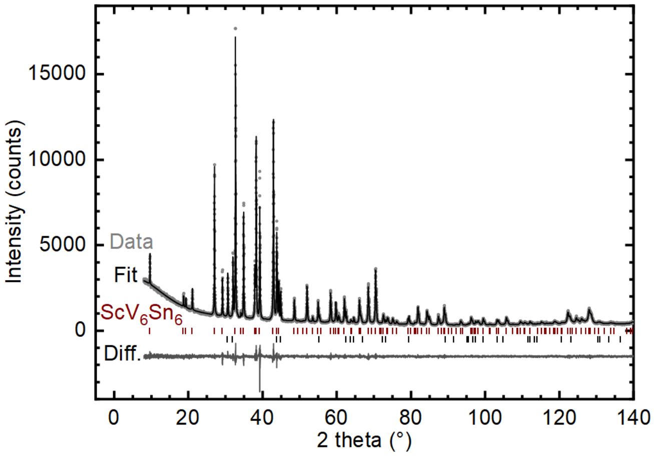


FIG. 2. Refined powder x-ray diffraction pattern from ground $ScV_6Sn_6$ crystals. Red ticks indicate peaks from $ScV_6Sn_6$ and black ticks beta-Sn (6 wt%).

TABLE I. Single crystal refinement data for $ScV_6Sn_6$ at 280 K.

| | |
|---|---|
| Temperature | 280 K |
| Refined formula | $ScV_6Sn_6$ |
| Formula weight (g/mol) | 1062.74 |
| Space group ; $Z$ | $P6/mmm$ (No. 191) ; 1 |
| $a$ (Å) | 5.46693(11) |
| $c$ (Å) | 9.1594(3) |
| $V$ (Å$^3$) | 237.074(12) |
| Extinction coeff. | 0.238(10) |
| Source ; wavelength (Å) | Mo $K_\alpha$ ; 0.71073 |
| $\theta$ range (°) | 2.224-33.239 |
| No. reflections ; $R_{\text{int}}$ | 5794 ; 0.0661 |
| No. independent reflections | 233 |
| No. parameters | 15 |
| $R_1$ ; $\omega R_2(I > 2\delta(I))$ | 0.0277 ; 0.0609 |
| Goodness of fit | 1.130 |

Another note on the high temperature single crystal refinement. The structure was refined with both Shelx [5, 6] and Jana [1] software. After further assessment of the refinement from each software it was found Shelx produced a higher-quality refinement, whereas Jana was

TABLE II. Single crystal refinement CDW superstructure for $ScV_6Sn_6$ at 50 K. *Method: B-C type 1 Gaussian isotropic [2]

| | |
|---|---|
| Temperature | 50 K |
| Refined formula | $ScV_6Sn_6$ |
| Formula weight (g/mol) | 1062.9 |
| Space group ; $Z$ | $R32$ (No. 155) ; 9 |
| $a$ (Å) | 9.4561(5) |
| $c$ (Å) | 27.4124(9) |
| $V$ (Å$^3$) | 2122.77(17) |
| Extinction coeff.* | 790(30) |
| Source ; wavelength (Å) | Mo $K_\alpha$ ; 0.71073 |
| $\theta$ range (°) | 2.23-33.51 |
| No. reflections ; $R_{\rm int}$ | 16785 ; 0.121 |
| No. independent reflections | 1737 |
| No. parameters | 63 |
| $R_1$ ; $\omega R_2(I > 2\delta(I))$ | 0.0381; 0.0467 |
| Goodness of fit | 1.03 |

TABLE III. Refined atomic coordinates for $ScV_6Sn_6$ at 280 K.

| Atom | Wyckoff | $x$ | $y$ | $z$ | $U_{\rm iso}$ |
|---|---|---|---|---|---|
| Sc1 | 1a | 0 | 0 | 0 | 0.0173(5) |
| V1 | 6i | $\frac{1}{2}$ | 0 | 0.24753(6) | 0.0095(3) |
| Sn1 | 2e | 0 | 0 | 0.32432(6) | 0.0143(2) |
| Sn2 | 2c | $\frac{1}{3}$ | $\frac{2}{3}$ | 0 | 0.0106(2) |
| Sn3 | 2d | $\frac{1}{3}$ | $\frac{2}{3}$ | $\frac{1}{2}$ | 0.0111(2) |

found to have issues with the calculated residual density. This difference is possibly related to Jana lacking the ability to refine certain parameters.

### Mössbauer spectroscopy

The $^{119}$Sn Mössbauer spectra of $ScV_6Sn_6$ are indicative of paramagnetic behavior between 6 and 300 K. The general shape of the spectra is a rather symmetric doublet, see Fig. 3. This observation indicates that all Sn sites, both in the low- and high-temperature phase have similar isomer shifts. The spectral shape reveals a clear modification in hyperfine interactions at about 90 K.

TABLE IV. Refined atomic coordinates for $ScV_6Sn_6$ at 50 K.

| Atom | Wyck. | $x$ | $y$ | $z$ | $U_{\rm iso}$ |
|---|---|---|---|---|---|
| Sc1 | 3a | 0 | 0 | 0 | 0.0079(6) |
| Sc1_2 | 6c | 0 | 0 | 0.32805(6) | 0.0085(4) |
| V1 | 18f | 0.3340(7) | 0.1672(7) | 0.08259(3) | 0.0062(8) |
| V1_2 | 18f | 0.1667(10) | 0.3333(7) | 0.08240(3) | 0.0063(8) |
| V1_3 | 18f | 0.1667(7) | 0.3329(10) | 0.25092(3) | 0.0063(8) |
| Sn1 | 6c | 0 | 0 | 0.10927(2) | 0.0071(2) |
| Sn1_2 | 6c | 0 | 0 | 0.22139(2) | 0.0076(2) |
| Sn1_3 | 6c | 0 | 0 | 0.43562(2) | 0.0080(2) |
| Sn2 | 9d | 0.33296(13) | 0 | 0 | 0.0036(3) |
| Sn2_2 | 9d | $\frac{2}{3}$ | 0.00000(16) | 0 | 0.0101(5) |
| Sn3 | 9e | 0.33231(14) | 0.00000(14) | $\frac{1}{2}$ | 0.0056(4) |
| Sn3_2 | 9e | 0.667770 | 0.00000(16) | $\frac{1}{2}$ | 0.0074(5) |

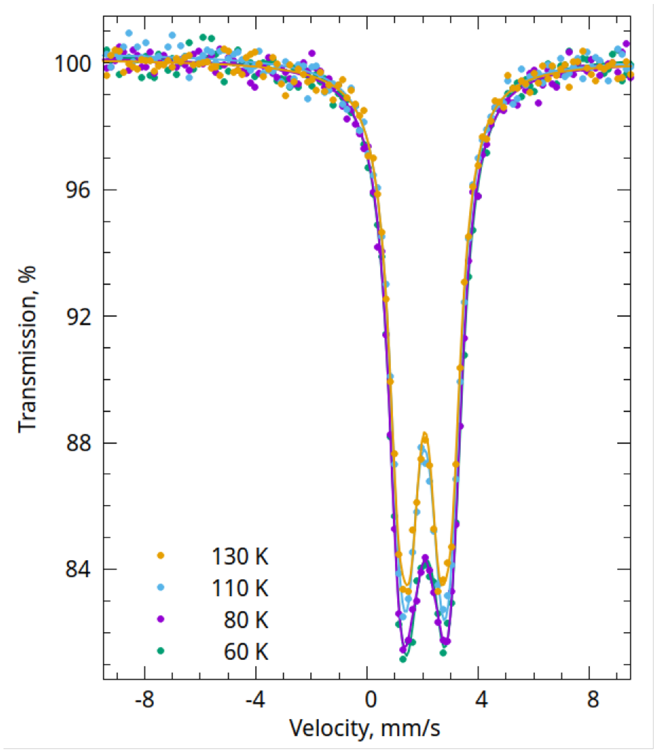


FIG. 3. Representative $^{119}Sn$ Mössbauer spectra of $ScV_6Sn_6$ accross the CDW transition with fitted as indicated in the text.

Preliminary fits showed that at least two doublets are needed to describe the data at any given temperature. This first analysis also revealed that robust modelling can be achieved by a phenomenological model which utilizes three principal components and only varies their relative amounts. The first component corresponds to a quadrupole splitting, $QS_1$, of 1.8 mm/s. This component is not affected by the CDW phase transition and was fixed at 63 % of the total spectral area. The second component had $QS_2 = 0.975$ mm/s and contributes 22 % of the spectral area at 295 K and $< 2$ % area at 6 K. The third component had $QS_3 = 0.73$ mm/s and contributes between 15 % spectral area at 295 K and 35 % at 6 K. The isomer shift for component 1 and 3, IS, was used as a free fit parameter and the isomer shift for component 2 was constrained to be 0.036 mm/s lower at any given temperature. The isomer shift decreases from 2.09(1) to 2.03(1) mm/s, relative to the $CaSnO_3$ source when heating from 6 to 295 K.

The deconvolution for the spectra is certainly not unique considering 3 Sn above and 9 sites below the CDW transition. All line widths are between 0.9 and 1.0 mm/s, which is also indicative of some distribution in spectral parameters. However, the principal component analysis based on only the relative area of component 2 and 3 adequately model all spectra and captures the essential

TABLE V. Refined anisotropic atomic displacement parameters, $U_{ij}$, for $ScV_6Sn_6$ at 280 K.

| Atom | $U_{11}$ | $U_{22}$ | $U_{33}$ | $U_{12}$ | $U_{13}$ | $U_{23}$ |
|---|---|---|---|---|---|---|
| Sc1 | 0.0134(6) | 0.0134(6) | 0.0252(12) | 0.0067(3) | 0 | 0 |
| V1 | 0.0100(3) | 0.0100(4) | 0.0087(4) | 0.0050(2) | 0 | 0 |
| Sn1 | 0.0102(3) | 0.0102(3) | 0.0224(4) | 0.00512(13) | 0 | 0 |
| Sn2 | 0.0114(3) | 0.0114(3) | 0.0090(3) | 0.00571(13) | 0 | 0 |
| Sn3 | 0.0122(3) | 0.0122(3) | 0.0089(3) | 0.00611(13) | 0 | 0 |

TABLE VI. Refined anisotropic atomic displacement parameters, $U_{ij}$, for $ScV_6Sn_6$ at 50 K.

| Atom | $U_{11}$ | $U_{22}$ | $U_{33}$ | $U_{12}$ | $U_{13}$ | $U_{23}$ |
|---|---|---|---|---|---|---|
| Sc1 | 0.0080(6) | 0.0080(6) | 0.0077(11) | 0.0040(3) | 0 | 0 |
| Sc1_2 | 0.0087(5) | 0.0087(5) | 0.0082(8) | 0.0044(2) | 0 | 0 |
| V1 | 0.0103(13) | 0.0050(12) | 0.0035(4) | 0.0039(3) | -0.0056(12) | -0.0020(12) |
| V1_2 | 0.0075(4) | 0.0096(13) | 0.0037(4) | 0.0058(13) | 0.0037(13) | 0.0017(12) |
| V1_3 | 0.0065(12) | 0.0077(4) | 0.0037(4) | 0.0029(12) | -0.0026(12) | -0.0039(13) |
| Sn1 | 0.0072(2) | 0.0072(2) | 0.0068(3) | 0.00360(10) | 0 | 0 |
| Sn1_2 | 0.0072(2) | 0.0072(2) | 0.0084(3) | 0.00360(10) | 0 | 0 |
| Sn1_3 | 0.0076(2) | 0.0076(2) | 0.0087(3) | 0.00380(10) | 0 | 0 |
| Sn2 | 0.0034(3) | 0.0075(5) | 0.0012(6) | 0.0038(2) | 0.0009(3) | 0.0018(5) |
| Sn2_2 | 0.0080(6) | 0.0129(5) | 0.0077(9) | 0.0040(3) | 0.0023(6) | 0.0012(3) |
| Sn3 | 0.0072(4) | 0.0072(4) | 0.0023(6) | 0.0036(4) | -0.0003(3) | 0.0003(3) |
| Sn3_2 | 0.0074(6) | 0.0079(5) | 0.0068(8) | 0.0037(3) | -0.0009(6) | -0.0004(3) |

changes in a single quantity, the average quadrupole splitting, as shown in Fig. 4c of the main text. This observation also indicates that the CDW transition is correlated with a significant change in the quadrupole splitting of roughly 1/3 of Sn atoms.

* ssuriyaa@vols.utk.edu
† javamocham@gmail.com
‡ dmandrus@utk.edu

[1] V. Petříček, M. Dušek, and L. Palatinus, Zeitschrift für Kristallographie - Crystalline Materials **229**, 345 (2014).
[2] P. J. Becker and P. Coppens, Acta Crystallographica Section A **30**, 129 (1974).
[3] H. T. Stokes, D. M. Hatch, and B. J. Campbell, ISODISTORT, ISOTROPY software suite, version 6.7.2 (Sep 2020).
[4] B. J. Campbell, H. T. Stokes, D. E. Tanner, and D. M. Hatch, Journal of Applied Crystallography **39**, 607 (2006).
[5] G. M. Sheldrick, Acta Crystallographica Section C Structural Chemistry **71**, 3 (2015).
[6] G. M. Sheldrick, Acta Crystallographica Section A Foundations and Advances **71**, 3 (2015).
